# Supplementary material for: The Untold Story of the Clones: Content-agnostic Factors that Impact YouTube Video Popularity
Source: arXiv:1311.6526 source file (2013-11-26)
Supplement: Supplementary file 1 [file appendix.tex]

\appendix

Below is a detailed description of the different sources of traffic for Youtube videos.

\begin{itemize}
        \item Ad:
The viewer was referred to the video through a paid Youtube promotion.
Videos can be promoted on the YouTube website through paid advertisement.
Such videos are labeled as ``Promoted Videos'' and appear next to related search results.
        \item Featured
The viewer was referred to the video through an unpaid Youtube promotion
such as the YouTube ``Featured Videos'' or ``Spotlight Videos'' sections.
It's interesting to note that most of the videos in the ``Featured Videos'' list
are selected from the ones uploaded by Youtube partners due to commercial advantages.
\item Mobile:
The video views occurred on a mobile device
through the mobile version of the Youtube website (m.youtube.com)
or through Youtube apps.
        \item Google Search: The viewer was referred to the video through
keyword searches on the Google search engine.
        \item YouTube Search
The viewer was referred to the video through keyword searches on YouTube.
        \item Related:
The viewer was referred to the video through related videos in YouTube.
        \item Embedded: The viewer was referred to the video through an embed on an external website.
%First embedded view: The video was embedded on another website when it was viewed.
        \item External: The viewer was referred to the video through links on other websites.
        \item Other/Viral: YouTube could not recognize a referrer for the views because the
the user navigated directly to the video by copying and pasting
the video's URL or by clicking on a link to the video from an email or instant message application.
        \item Youtube other (Internal):
The viewer was referred to the video through a Youtube link other than
a related video or search result. Other pages on YouTube could be
the YouTube homepage, category pages, a user profile page,
other peoples channel pages and a user generated playlist.
        \item Subscriber:
The video views occurred as a result of the uploader channel's subscribers clicking on
it in one of the subscription notification modules.
        \item Channel:
The video views occurred on the uploader's channel page.
\end{itemize}
